# Supplementary material for: A study of $C\!P$ violation in the decays $B^\pm\to[K^+K^-\pi^+\pi^-]_D h^{\pm}$ ($h = K, \pi$) and $B^\pm\to[\pi^+\pi^-\pi^+\pi^-]_D h^{\pm}$
Source: arXiv:2301.10328 source file (2023-07-31)
Supplement: Supplementary file 1 [file supplementary-app.tex]

\clearpage

\section{Supplementary material for LHCb-PAPER-2022-037}
\label{sec:Supplementary-App}

The invariant-mass fit of $\Bpm\to[\Kp\Km\pip\pim]_\Dh^\pm$ is shown in Fig.~\ref{Global_fit_log} on a logarithmic scale, where the individual background components can be seen more clearly.

\begin{figure}[!htb]
    \centering
    \includegraphics[width=1.0\textwidth]{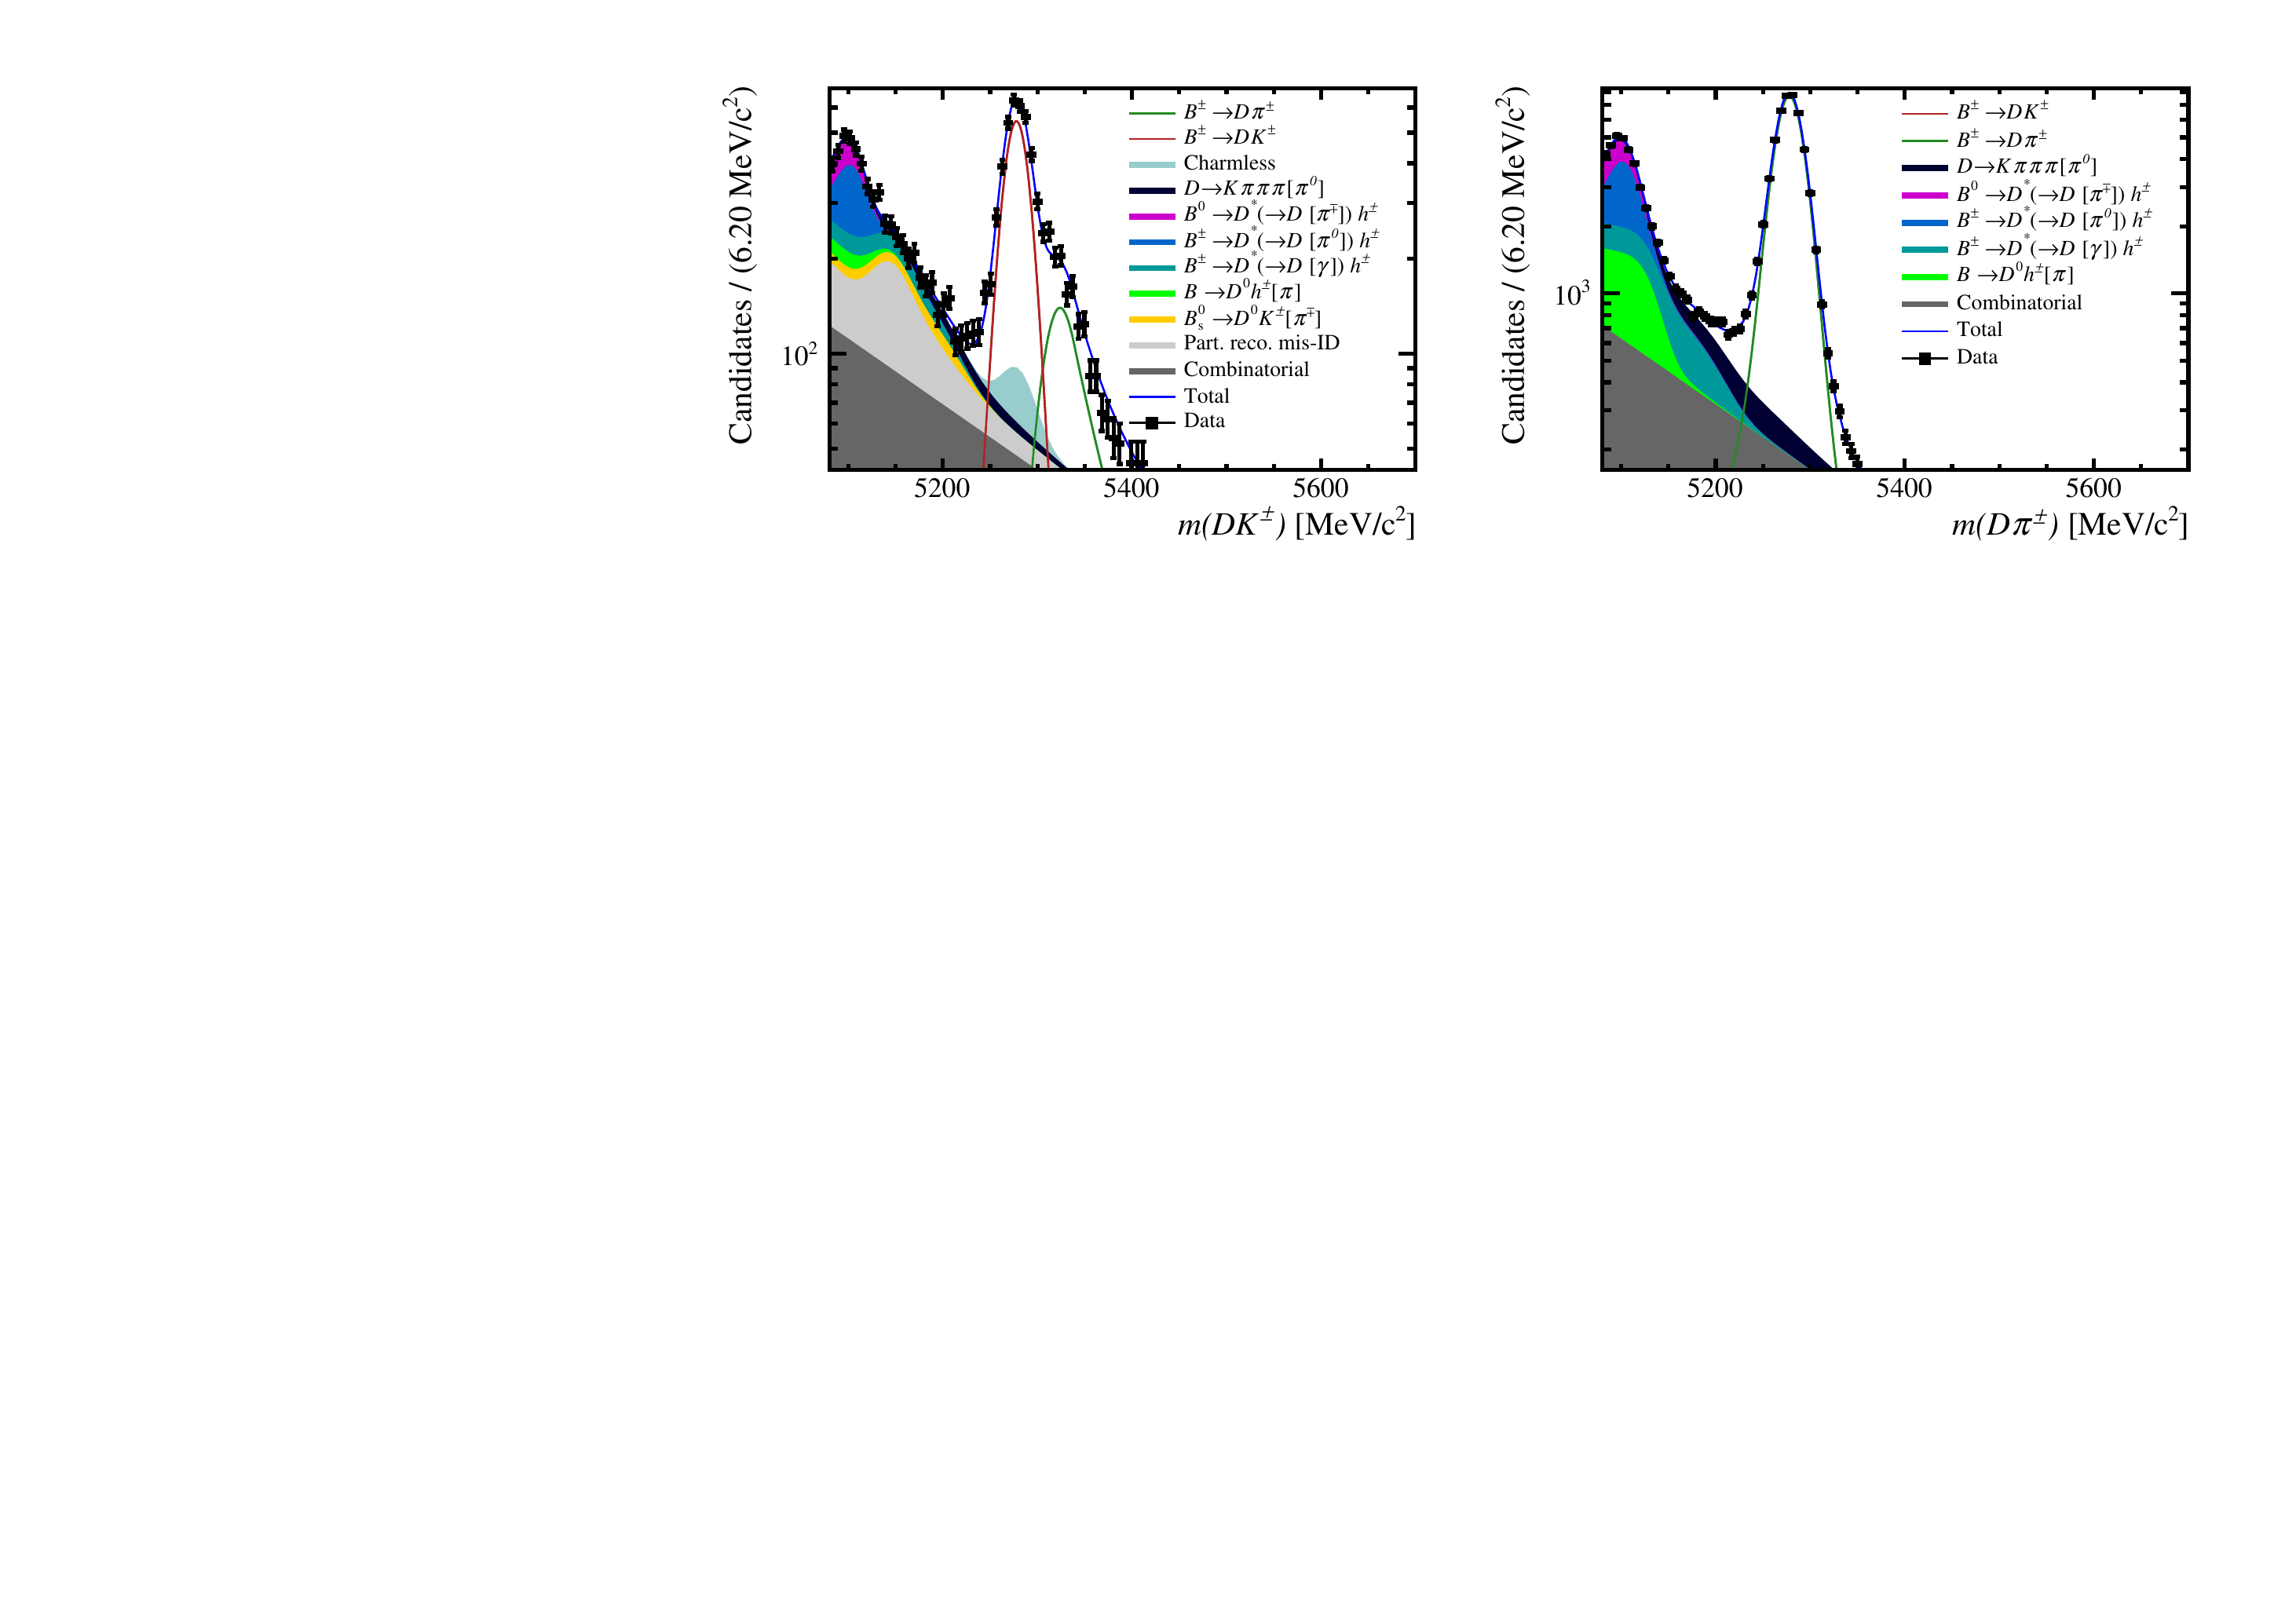}
    \caption{Invariant-mass distributions on a logarithmic scale for the (left) $\Bpm\to\D\Kpm$ and (right) $\Bpm\to\D\pipm$ selections, for the $\D\to\Kp\Km\pip\pim$ decay. The data are shown as black points and the blue curve is the fit result. The square brackets in the legend denote particles that are not reconstructed. The range on the vertical axis has been chosen to allow for the different contributions in the low mass background to be clearly visualised.}
    \label{figure:Global_fit_log}
\end{figure}

\clearpage
